# Supplementary material for: Decision support from financial disclosures with deep neural networks and transfer learning
Source: arXiv:1710.03954 ancillary file (2017-10-11)
Supplement: Supplementary file 1 [file online_appendix.pdf]

## Appendix A. Tuning parameters

Table A.1 reports the tuning parameters used in our grid search.

| Predictive model | Tuning parameters | Tuning range | Final parameter choice | | | |
|---|---|---|---|---|---|---|
| | | | C/R | C/AR | R/R | R/AR |
| Ridge regression | Regularization strength $\alpha$ | 1, 0.99, 0.95, 0.9, ..., 0.1, 0.05, 0.01 | 0.9 | 0.99 | 0.9 | 0.85 |
| | Number $n_{\max}$ of selected features | 200, 300, 400, 500, 1000, all | 300 | 400 | 500 | 500 |
| | Stemming | enabled, disabled | enabled | disabled | enabled | enabled |
| Lasso | Regularization strength $\alpha$ | 1, 0.99, 0.95, 0.9, ..., 0.1, 0.05, 0.01 | — | — | 0.9 | 0.8 |
| | Number $n_{\max}$ of selected features | 200, 300, 400, 500, 1000, all | — | — | all | 1000 |
| | Stemming | enabled, disabled | — | — | enabled | enabled |
| Elastic net | Ratio of $L_1$- and $L_2$-penalties $\alpha_1$, $\alpha_2$ | 1, 0.99, 0.95, 0.9, ..., 0.1, 0.05, 0.01 | — | — | 0.95 | 0.95 |
| | Number $n_{\max}$ of selected features | 200, 300, 400, 500, 1000, all | — | — | 500 | 500 |
| | Stemming | enabled, disabled | — | — | enabled | enabled |
| Random forest | Number of randomly-sampled variables | 1, 2, 3, 5, 7 | 3 | 5 | 3 | 2 |
| | Number of trees | 100, 200, 500, 1000 | 1000 | 500 | 200 | 500 |
| | Maximum depth of trees | 1, 5, 10, 20, 50, 100, None | None | 20 | None | 100 |
| | Number $n_{\max}$ of selected features | 200, 300, 400, 500, 1000, all | 400 | all | 300 | 300 |
| | Stemming | enabled, disabled | disabled | disabled | enabled | enabled |
| AdaBoost | Maximum number of trees | 1, 5, 10, 20, 50, 100 | 50 | 100 | 50 | 20 |
| | Learning rate | 1, 0.99, 0.95, 0.9, ..., 0.1, 0.05, 0.01 | 0.15 | 0.2 | 0.05 | 0.05 |
| | Number $n_{\max}$ of selected features | 200, 300, 400, 500, 1000† | 1000 | all | 300 | 300 |
| | Stemming | enabled, disabled | enabled | enabled | enabled | enabled |
| Gradient boosting | Maximum number of weak learners | 100, 200, 500, 1000 | 500 | 200 | 100 | 200 |
| | Loss function | [least squares, least absolute, huber] | least squares | least squares | least squares | least squares |
| | Learning rate | 1, 0.99, 0.95, 0.9, ..., 0.1, 0.05, 0.01 | 0.1 | 0.05 | 0.1 | 0.1 |
| | Number $n_{\max}$ of selected features | 200, 300, 400, 500† | 300 | 400 | 200 | 300 |
| | Stemming | enabled, disabled | enabled | enabled | enabled | enabled |
| SVM | Kernel function | Linear, radial, poly | linear | linear | radial | radial |
| | Cost $C$ | 1.0, 0.99, 0.95, 0.9, ..., 0.1, 0.05, 0.01 | 0.15 | 0.15 | 0.05 | 0.1 |
| | Number $n_{\max}$ of selected features | 200, 300, 400, 500, 1000, all | 300 | 200 | 200 | 500 |
| | Stemming | enabled, disabled | enabled | disabled | enabled | disabled |
| RNN | Word embedding size | 30, 40, ..., 100 | 40 | 30 | 50 | 40 |
| | Learning rate | 0.0001, 0.0005, ..., 0.0095, 0.01 | 0.0005 | 0.0005 | 0.005 | 0.001 |
| | Stemming | enabled, disabled | disabled | disabled | disabled | disabled |
| LSTM | Word embedding size | 30, 40, ..., 100 | 50 | 40 | 60 | 60 |
| | Learning rate | 0.0001, 0.0005, ..., 0.0095, 0.01 | 0.0005 | 0.005 | 0.001 | 0.001 |
| | Stemming | enabled, disabled | disabled | disabled | disabled | disabled |
| LSTM with word embeddings | Word embedding size | 30, 40, ..., 100 | 60 | 70 | 70 | 50 |
| | Learning rate | 0.0001, 0.0005, ..., 0.0095, 0.01 | 0.01 | 0.005 | 0.005 | 0.005 |
| | Stemming | enabled, disabled | disabled | disabled | disabled | disabled |

† Skipped larger values due to high computational time

Table A.1: Parameters tuned via time-series cross-validation in order to find the best model. Here we refer to the different experiments as follows: classification with nominal returns (C/R) and abnormal returns (C/AR); regression with nominal (R/R) and abnormal returns (R/AR).

## Appendix B. Sensitivity analysis: *n*-grams

In the following, Table B.2 shows the effect of utilizing bigrams within traditional machine learning models (with stemming only) to classify the direction of abnormal return. As a result, ridge regression performs best across all approaches and metrics, outperforming the naïve approach by 4.8 percentage points in terms of balanced accuracy. Among non-linear models, random forest performs best with a balanced accuracy of 54.1 %, amounting to an increased performance of 4.1 percentage points. Overall, we observe no clear evidence that either unigrams or bigrams performs better.

| **Method** | **Training set** | **Test set** | | |
|---|---|---|---|---|
| | **Accuracy** | **Accuracy** | **Balanced accuracy** | **AUC** |
| Naïve baseline (majority class) | 0.542 | 0.528 | 0.500 | 0.500 |
| Ridge regression | 0.540 | **0.552** | **0.548** | **0.560** |
| Lasso | 0.542 | 0.528 | 0.500 | 0.500 |
| Elastic net | 0.542 | 0.528 | 0.500 | 0.500 |
| Random Forest | **0.554** | 0.548 | 0.541 | 0.555 |
| SVM | 0.548 | 0.536 | 0.523 | 0.549 |
| AdaBoost | 0.547 | 0.535 | 0.525 | 0.551 |
| Gradient Boosting | 0.552 | 0.535 | 0.514 | 0.534 |

Table B.2: Out-of-sample results from baselines utilizing bigrams to classify the direction of abnormal return.

Table B.3 reports the results of traditional models with stemming only when incorporating trigrams. Again, ridge regression and random forest perform well, beating the naïve benchmark by 4.1 and 4.0 percentage points, respectively. Again, there is no direct recommendation on whether to prefer unigrams or trigrams

| **Method** | **Training set** | **Test set** | | |
|---|---|---|---|---|
| | **Accuracy** | **Accuracy** | **Balanced accuracy** | **AUC** |
| Naïve baseline (majority class) | 0.542 | 0.528 | 0.500 | 0.500 |
| Ridge regression | 0.538 | 0.545 | **0.541** | **0.565** |
| Lasso | 0.542 | 0.528 | 0.500 | 0.500 |
| Elastic net | 0.542 | 0.528 | 0.500 | 0.500 |
| Random Forest | **0.554** | **0.547** | 0.540 | 0.552 |
| SVM | 0.547 | 0.540 | 0.527 | 0.549 |
| AdaBoost | 0.544 | 0.541 | 0.532 | 0.552 |
| Gradient Boosting | 0.552 | 0.537 | 0.516 | 0.536 |

Table B.3: Out-of-sample results from baselines utilizing trigrams to classify the direction of abnormal return.

## Appendix C. Explanatory insights for finance-specific words

Table C.4 and Table C.5 report the standardized results of the LSTM for classifying abnormal returns with pre-training and word embeddings when predicting sentiment scores of single words from the Loughran-McDonald dictionary [1]. We observe several differences across inflected word forms. This is partially owed to the fact that these words are not part of Glove and thus become initialized randomly. We thus repeat the analysis with an LSTM that is trained on word stems; see Table C.6 and Table C.7.

### *Appendix C.1. Inflected words*

| **Entry** | **Label** | **Predicted score** |
|---|---|---|
| achieve | Positive | 0.338 |
| achieved | Positive | 0.478 |
| achievement | Positive | 0.282 |
| achievements | Positive | 0.216 |
| achieves | Positive | 0.080 |
| achieving | Positive | 0.054 |
| adequately | Positive | 0.284 |
| advances | Positive | 0.022 |
| advancing | Positive | 0.102 |
| advantage | Positive | 0.256 |
| advantageous | Positive | −0.174 |
| advantages | Positive | −0.070 |
| alliance | Positive | 0.164 |
| alliances | Positive | 0.114 |
| assure | Positive | −0.102 |
| assured | Positive | 0.020 |
| attain | Positive | 0.206 |
| attained | Positive | 0.102 |
| attractive | Positive | 0.580 |
| attractiveness | Positive | 0.286 |
| beneficial | Positive | 0.380 |
| benefit | Positive | 0.194 |
| benefited | Positive | 0.076 |
| benefiting | Positive | −0.282 |
| best | Positive | 0.264 |
| better | Positive | 0.184 |
| boom | Positive | −0.002 |
| booming | Positive | 0.012 |
| boost | Positive | 0.274 |
| boosted | Positive | −0.004 |
| breakthrough | Positive | 0.096 |
| collaboration | Positive | −0.346 |
| collaborations | Positive | 0.194 |

| | | |
|---|---|---|
| confident | Positive | 0.046 |
| constructive | Positive | 0.562 |
| creative | Positive | 0.350 |
| delighted | Positive | 0.106 |
| desired | Positive | −0.040 |
| despite | Positive | 0.122 |
| easier | Positive | 0.310 |
| easily | Positive | −0.250 |
| easy | Positive | −0.156 |
| effective | Positive | 0.428 |
| efficiencies | Positive | 0.198 |
| efficiency | Positive | 0.420 |
| efficient | Positive | −0.040 |
| efficiently | Positive | 0.100 |
| enable | Positive | 0.024 |
| enabled | Positive | −0.094 |
| enables | Positive | 0.172 |
| enabling | Positive | 0.030 |
| encouraged | Positive | −0.200 |
| encourages | Positive | 0.156 |
| encouraging | Positive | 0.316 |
| enhance | Positive | −0.090 |
| enhanced | Positive | 0.138 |
| enhancement | Positive | −0.062 |
| enhancements | Positive | 0.026 |
| enhances | Positive | 0.122 |
| enhancing | Positive | 0.326 |
| enjoy | Positive | 0.223 |
| enjoyable | Positive | 0.065 |
| enjoyed | Positive | −0.198 |
| enjoying | Positive | 0.009 |
| enjoyment | Positive | 0.190 |
| enjoys | Positive | −0.273 |
| enthusiasm | Positive | −0.163 |
| enthusiastic | Positive | 0.237 |
| excellence | Positive | 0.140 |
| excellent | Positive | −0.021 |
| excels | Positive | −0.117 |
| exceptional | Positive | 0.006 |
| exceptionally | Positive | 0.033 |
| excited | Positive | 0.170 |
| excitement | Positive | 0.080 |
| exciting | Positive | 0.132 |
| exclusive | Positive | 0.587 |
| exclusively | Positive | 0.046 |
| exclusivity | Positive | 0.148 |
| exemplary | Positive | 0.389 |
| fantastic | Positive | 0.292 |
| favorable | Positive | −0.323 |

| | | |
|---|---|---|
| favorably | Positive | 0.346 |
| favored | Positive | 0.137 |
| favoring | Positive | 0.287 |
| favorite | Positive | 0.124 |
| friendly | Positive | −0.118 |
| gain | Positive | −0.103 |
| gained | Positive | −0.152 |
| gaining | Positive | −0.039 |
| gains | Positive | 0.302 |
| good | Positive | −0.093 |
| great | Positive | 0.318 |
| greater | Positive | −0.049 |
| greatest | Positive | 0.002 |
| greatly | Positive | −0.402 |
| happily | Positive | 0.033 |
| happiness | Positive | 0.291 |
| happy | Positive | 0.073 |
| highest | Positive | 0.396 |
| honor | Positive | 0.092 |
| honored | Positive | −0.036 |
| honoring | Positive | 0.039 |
| honors | Positive | −0.093 |
| ideal | Positive | 0.263 |
| impressed | Positive | 0.045 |
| impresses | Positive | 0.268 |
| impressing | Positive | −0.277 |
| impressive | Positive | −0.092 |
| impressively | Positive | −0.517 |
| improve | Positive | 0.070 |
| improved | Positive | −0.313 |
| improvement | Positive | −0.158 |
| improvements | Positive | 0.252 |
| improves | Positive | −0.124 |
| improving | Positive | −0.363 |
| incredible | Positive | −0.016 |
| informative | Positive | −0.204 |
| innovate | Positive | −0.221 |
| innovating | Positive | 0.042 |
| innovation | Positive | 0.273 |
| innovations | Positive | 0.045 |
| innovative | Positive | −0.103 |
| innovativeness | Positive | −0.018 |
| innovator | Positive | 0.524 |
| insightful | Positive | −0.350 |
| integrity | Positive | 0.014 |
| invented | Positive | −0.369 |
| invention | Positive | 0.300 |
| inventive | Positive | 0.211 |
| inventor | Positive | 0.272 |

| | | |
|---|---|---|
| leadership | Positive | 0.331 |
| leading | Positive | −0.110 |
| loyal | Positive | −0.148 |
| lucrative | Positive | 0.177 |
| opportunities | Positive | 0.117 |
| opportunity | Positive | 0.445 |
| optimistic | Positive | 0.114 |
| outperform | Positive | 0.257 |
| outperformed | Positive | 0.348 |
| outperforming | Positive | −0.036 |
| outperforms | Positive | −0.226 |
| perfect | Positive | 0.437 |
| perfectly | Positive | −0.024 |
| pleasant | Positive | 0.189 |
| pleasantly | Positive | 0.178 |
| pleased | Positive | 0.339 |
| pleasure | Positive | 0.059 |
| popular | Positive | 0.061 |
| popularity | Positive | 0.044 |
| positive | Positive | −0.147 |
| positively | Positive | −0.016 |
| premier | Positive | 0.209 |
| premiere | Positive | −0.167 |
| prestige | Positive | 0.196 |
| prestigious | Positive | −0.078 |
| proactive | Positive | 0.279 |
| proactively | Positive | 0.124 |
| profitability | Positive | 0.255 |
| profitable | Positive | −0.099 |
| profitably | Positive | −0.177 |
| progress | Positive | 0.231 |
| progressed | Positive | 0.307 |
| progresses | Positive | −0.029 |
| progressing | Positive | 0.323 |
| prospered | Positive | −0.118 |
| prospering | Positive | −0.088 |
| prosperity | Positive | 0.386 |
| prosperous | Positive | −0.017 |
| rebound | Positive | 0.020 |
| rebounded | Positive | 0.090 |
| rebounding | Positive | −0.002 |
| regain | Positive | 0.195 |
| regained | Positive | −0.101 |
| regaining | Positive | −0.123 |
| resolve | Positive | 0.345 |
| revolutionize | Positive | 0.180 |
| revolutionizing | Positive | 0.375 |
| reward | Positive | 0.090 |
| rewarded | Positive | 0.088 |

| | | |
|---|---|---|
| rewarding | Positive | 0.212 |
| rewards | Positive | 0.297 |
| satisfaction | Positive | −0.070 |
| satisfactorily | Positive | 0.108 |
| satisfactory | Positive | 0.124 |
| satisfied | Positive | 0.219 |
| satisfies | Positive | 0.341 |
| satisfy | Positive | −0.221 |
| satisfying | Positive | 0.298 |
| smooth | Positive | 0.155 |
| smoothly | Positive | 0.109 |
| solves | Positive | −0.098 |
| solving | Positive | 0.057 |
| spectacular | Positive | 0.236 |
| stability | Positive | −0.086 |
| stabilization | Positive | −0.071 |
| stabilize | Positive | 0.466 |
| stabilized | Positive | −0.043 |
| stabilizes | Positive | 0.144 |
| stabilizing | Positive | 0.399 |
| stable | Positive | 0.085 |
| strength | Positive | 0.499 |
| strengthen | Positive | 0.259 |
| strengthened | Positive | 0.041 |
| strengthening | Positive | 0.129 |
| strengthens | Positive | 0.088 |
| strengths | Positive | 0.160 |
| strong | Positive | 0.252 |
| stronger | Positive | 0.361 |
| strongest | Positive | −0.383 |
| succeed | Positive | −0.052 |
| succeeded | Positive | −0.099 |
| succeeding | Positive | −0.041 |
| succeeds | Positive | 0.372 |
| success | Positive | 0.028 |
| successes | Positive | 0.180 |
| successful | Positive | 0.111 |
| successfully | Positive | −0.384 |
| superior | Positive | 0.234 |
| surpass | Positive | 0.337 |
| surpassed | Positive | −0.097 |
| surpasses | Positive | 0.086 |
| surpassing | Positive | 0.054 |
| transparency | Positive | 0.014 |
| tremendous | Positive | 0.232 |
| tremendously | Positive | −0.440 |
| unparalleled | Positive | −0.214 |
| upturn | Positive | 0.132 |
| valuable | Positive | 0.003 |

| | | |
|---|---|---|
| versatile | Positive | 0.198 |
| versatility | Positive | −0.138 |
| vibrant | Positive | −0.181 |
| win | Positive | 0.109 |
| winner | Positive | 0.548 |
| winners | Positive | 0.350 |
| winning | Positive | −0.054 |
| worthy | Positive | 0.178 |

Table C.4: Standardized predictions for all positive terms from the Loughran-McDonald finance-specific word list. The results stem from an LSTM with word embeddings for the regression task with abnormal returns.

| **Entry** | **Label** | **Predicted score** |
|---|---|---|
| absence | Negative | −0.176 |
| abuse | Negative | −0.034 |
| adverse | Negative | 0.028 |
| adversely | Negative | −0.136 |
| against | Negative | −0.092 |
| allegations | Negative | −0.214 |
| alleged | Negative | −0.444 |
| antitrust | Negative | 0.588 |
| bad | Negative | 0.030 |
| bankruptcy | Negative | −0.158 |
| bottlenecks | Negative | −0.058 |
| breach | Negative | −0.124 |
| break | Negative | −0.500 |
| breakdown | Negative | −0.126 |
| breaking | Negative | −0.198 |
| bridge | Negative | 0.012 |
| burden | Negative | −0.350 |
| burdened | Negative | −0.094 |
| burdening | Negative | −0.122 |
| burdens | Negative | −0.140 |
| cancel | Negative | 0.210 |
| canceled | Negative | −0.002 |
| canceling | Negative | 0.021 |
| cancellation | Negative | −0.184 |
| caution | Negative | 0.002 |
| cautionary | Negative | −0.278 |
| cautioned | Negative | −0.016 |
| cease | Negative | −0.318 |
| ceased | Negative | −0.096 |
| challenge | Negative | −0.456 |
| challenges | Negative | −0.102 |

| | | |
|---|---|---|
| challenging | Negative | −0.018 |
| claims | Negative | −0.302 |
| closed | Negative | −0.156 |
| closing | Negative | −0.220 |
| closure | Negative | 0.038 |
| closures | Negative | 0.058 |
| collapse | Negative | 0.014 |
| complaint | Negative | −0.034 |
| concern | Negative | 0.044 |
| concerned | Negative | 0.128 |
| concerns | Negative | 0.086 |
| conflict | Negative | −0.156 |
| contraction | Negative | 0.018 |
| contrary | Negative | −0.130 |
| corrected | Negative | 0.064 |
| correction | Negative | 0.032 |
| corrections | Negative | 0.044 |
| criminal | Negative | −0.044 |
| crises | Negative | −0.136 |
| crisis | Negative | −0.105 |
| critical | Negative | 0.005 |
| critically | Negative | −0.263 |
| criticism | Negative | 0.084 |
| criticisms | Negative | −0.007 |
| crucial | Negative | −0.107 |
| crucially | Negative | 0.185 |
| culpably | Negative | 0.009 |
| curtail | Negative | 0.050 |
| curtailed | Negative | −0.135 |
| curtailing | Negative | 0.111 |
| curtailment | Negative | −0.085 |
| curtailments | Negative | −0.003 |
| cut | Negative | 0.103 |
| cutback | Negative | 0.146 |
| cutbacks | Negative | 0.218 |
| damage | Negative | −0.267 |
| damaged | Negative | −0.306 |
| damages | Negative | −0.143 |
| damaging | Negative | 0.096 |
| dampen | Negative | 0.218 |
| dampened | Negative | 0.245 |
| danger | Negative | 0.019 |
| dangerous | Negative | −0.120 |
| dangers | Negative | −0.020 |
| deadlocks | Negative | −0.086 |
| deceit | Negative | 0.175 |
| deceptively | Negative | −0.040 |
| decline | Negative | −0.323 |
| declined | Negative | 0.058 |

| | | |
|---|---|---|
| declines | Negative | 0.099 |
| declining | Negative | 0.022 |
| defamatory | Negative | 0.058 |
| default | Negative | −0.211 |
| defaults | Negative | −0.132 |
| defeat | Negative | 0.026 |
| defeated | Negative | −0.097 |
| defective | Negative | −0.027 |
| defects | Negative | 0.087 |
| defend | Negative | −0.362 |
| defendant | Negative | −0.371 |
| defendants | Negative | 0.071 |
| defended | Negative | −0.183 |
| defer | Negative | 0.277 |
| deficiencies | Negative | 0.059 |
| deficiency | Negative | 0.097 |
| deficit | Negative | −0.024 |
| deficits | Negative | 0.067 |
| defrauded | Negative | 0.098 |
| defrauding | Negative | 0.225 |
| defunct | Negative | −0.287 |
| degradation | Negative | −0.401 |
| delay | Negative | 0.051 |
| delayed | Negative | 0.380 |
| delaying | Negative | 0.201 |
| delays | Negative | 0.314 |
| deliberate | Negative | −0.006 |
| deliberated | Negative | −0.119 |
| deliberately | Negative | 0.103 |
| delist | Negative | 0.012 |
| delisted | Negative | 0.588 |
| delisting | Negative | −0.220 |
| demolished | Negative | −0.106 |
| demolition | Negative | −0.064 |
| denied | Negative | 0.212 |
| denies | Negative | 0.019 |
| deny | Negative | −0.124 |
| depleted | Negative | 0.080 |
| depletion | Negative | 0.278 |
| deprecation | Negative | 0.048 |
| depress | Negative | 0.113 |
| depressed | Negative | −0.009 |
| depressing | Negative | −0.216 |
| deprive | Negative | −0.092 |
| deprived | Negative | −0.090 |
| destabilize | Negative | −0.234 |
| destroyed | Negative | −0.074 |
| destroys | Negative | 0.223 |
| destruction | Negative | 0.162 |

| | | |
|---|---|---|
| destructive | Negative | 0.299 |
| detain | Negative | 0.278 |
| detention | Negative | −0.096 |
| deter | Negative | 0.176 |
| deteriorate | Negative | 0.373 |
| deteriorated | Negative | −0.041 |
| deteriorates | Negative | −0.217 |
| deteriorating | Negative | −0.354 |
| deterioration | Negative | 0.064 |
| deteriorations | Negative | −0.136 |
| deterrent | Negative | 0.209 |
| detract | Negative | 0.197 |
| detracted | Negative | 0.193 |
| detriment | Negative | 0.213 |
| detrimental | Negative | 0.094 |
| devastating | Negative | −0.154 |
| devastation | Negative | 0.223 |
| deviate | Negative | 0.098 |
| deviated | Negative | 0.069 |
| deviates | Negative | 0.178 |
| deviating | Negative | 0.193 |
| deviation | Negative | 0.095 |
| deviations | Negative | −0.165 |
| difficult | Negative | −0.034 |
| difficulties | Negative | 0.081 |
| difficulty | Negative | 0.137 |
| diminish | Negative | −0.173 |
| diminished | Negative | 0.272 |
| diminishes | Negative | 0.234 |
| diminishing | Negative | 0.124 |
| diminution | Negative | −0.130 |
| disadvantage | Negative | −0.208 |
| disadvantaged | Negative | 0.281 |
| disadvantageous | Negative | 0.063 |
| disadvantages | Negative | −0.021 |
| disagreement | Negative | 0.159 |
| disagreements | Negative | −0.085 |
| disagrees | Negative | 0.067 |
| disappear | Negative | −0.541 |
| disappeared | Negative | −0.016 |
| disappointed | Negative | −0.308 |
| disappointing | Negative | 0.053 |
| disappointment | Negative | −0.080 |
| disapproval | Negative | 0.051 |
| disaster | Negative | 0.022 |
| disasters | Negative | −0.120 |
| disastrous | Negative | 0.122 |
| disciplinary | Negative | 0.105 |
| disclaim | Negative | 0.265 |

| | | |
|---|---|---|
| disclaimed | Negative | −0.347 |
| disclaimer | Negative | −0.261 |
| disclaims | Negative | 0.056 |
| disclose | Negative | 0.023 |
| disclosed | Negative | 0.148 |
| discloses | Negative | 0.029 |
| disclosing | Negative | 0.026 |
| discontinuance | Negative | 0.104 |
| discontinuation | Negative | −0.395 |
| discontinue | Negative | 0.239 |
| discontinued | Negative | 0.201 |
| discontinues | Negative | −0.002 |
| discontinuing | Negative | −0.221 |
| discrepancies | Negative | −0.574 |
| discrepancy | Negative | −0.367 |
| disgorgement | Negative | −0.284 |
| dismiss | Negative | −0.187 |
| dismissal | Negative | −0.021 |
| dismissals | Negative | −0.098 |
| dismissed | Negative | 0.020 |
| dismisses | Negative | −0.197 |
| dismissing | Negative | 0.153 |
| displace | Negative | −0.187 |
| displacement | Negative | 0.057 |
| displacing | Negative | 0.043 |
| dispose | Negative | −0.097 |
| disproportion | Negative | 0.007 |
| disproportional | Negative | −0.157 |
| disproportionate | Negative | −0.147 |
| disproportionately | Negative | −0.157 |
| dispute | Negative | −0.059 |
| disputed | Negative | 0.244 |
| disputes | Negative | 0.119 |
| disqualification | Negative | −0.088 |
| disqualified | Negative | 0.055 |
| disregarding | Negative | −0.088 |
| disrupt | Negative | 0.021 |
| disrupted | Negative | 0.123 |
| disrupting | Negative | 0.001 |
| disruption | Negative | −0.204 |
| disruptions | Negative | −0.170 |
| disruptive | Negative | −0.616 |
| dissatisfaction | Negative | 0.710 |
| dissent | Negative | −0.027 |
| dissented | Negative | 0.055 |
| dissenting | Negative | 0.130 |
| dissolution | Negative | 0.129 |
| distort | Negative | 0.090 |
| distorted | Negative | −0.365 |

| | | |
|---|---|---|
| distortion | Negative | 0.187 |
| distortions | Negative | 0.171 |
| distraction | Negative | 0.193 |
| distress | Negative | −0.162 |
| distressed | Negative | 0.274 |
| disturbances | Negative | −0.118 |
| disturbed | Negative | 0.215 |
| disturbing | Negative | 0.027 |
| divest | Negative | −0.126 |
| divested | Negative | 0.188 |
| divesting | Negative | −0.089 |
| divestiture | Negative | 0.141 |
| divestitures | Negative | 0.216 |
| divestment | Negative | 0.101 |
| divestments | Negative | −0.056 |
| divests | Negative | −0.050 |
| divulge | Negative | 0.284 |
| doubt | Negative | 0.163 |
| doubtful | Negative | 0.013 |
| doubts | Negative | −0.151 |
| downgrade | Negative | 0.155 |
| downgraded | Negative | −0.008 |
| downgrades | Negative | 0.367 |
| downsize | Negative | 0.071 |
| downsized | Negative | −0.002 |
| downsizing | Negative | 0.010 |
| downtime | Negative | 0.180 |
| downtimes | Negative | 0.077 |
| downturn | Negative | 0.090 |
| downturns | Negative | 0.164 |
| downward | Negative | −0.258 |
| downwards | Negative | 0.014 |
| drag | Negative | −0.098 |
| drastic | Negative | −0.266 |
| drastically | Negative | −0.183 |
| drawbacks | Negative | 0.100 |
| dropped | Negative | −0.057 |
| drought | Negative | 0.305 |
| dysfunction | Negative | 0.031 |
| easing | Negative | −0.083 |
| embarrassment | Negative | 0.087 |
| encumbered | Negative | −0.201 |
| encumbering | Negative | 0.019 |
| encumbrance | Negative | −0.022 |
| encumbrances | Negative | −0.051 |
| endanger | Negative | 0.307 |
| endangered | Negative | −0.043 |
| endangering | Negative | 0.027 |
| enjoining | Negative | 0.171 |

| | | |
|---|---|---|
| erode | Negative | −0.046 |
| eroded | Negative | 0.006 |
| eroding | Negative | −0.362 |
| erosion | Negative | −0.015 |
| erroneous | Negative | 0.258 |
| error | Negative | −0.177 |
| errors | Negative | −0.048 |
| escalate | Negative | 0.018 |
| escalated | Negative | −0.267 |
| escalating | Negative | 0.113 |
| exacerbated | Negative | 0.130 |
| exacerbations | Negative | 0.081 |
| exaggerated | Negative | 0.266 |
| excessive | Negative | 0.069 |
| excessively | Negative | −0.140 |
| exonerated | Negative | 0.250 |
| exonerates | Negative | 0.243 |
| exonerating | Negative | −0.053 |
| exploit | Negative | −0.185 |
| exploitation | Negative | 0.229 |
| exploited | Negative | 0.242 |
| exploiting | Negative | 0.027 |
| exposed | Negative | −0.033 |
| expulsion | Negative | 0.216 |
| fail | Negative | 0.028 |
| failed | Negative | 0.131 |
| failing | Negative | −0.534 |
| fails | Negative | 0.083 |
| failure | Negative | −0.096 |
| failures | Negative | −0.137 |
| 0 | Negative | −0.054 |
| fault | Negative | 0.190 |
| faults | Negative | −0.119 |
| faulty | Negative | −0.172 |
| fears | Negative | 0.153 |
| felony | Negative | −0.284 |
| fictitious | Negative | −0.401 |
| fines | Negative | 0.208 |
| fired | Negative | −0.129 |
| firing | Negative | 0.129 |
| flaws | Negative | 0.088 |
| forbid | Negative | −0.053 |
| forbidden | Negative | −0.064 |
| forbids | Negative | −0.058 |
| force | Negative | 0.190 |
| forced | Negative | 0.107 |
| forego | Negative | 0.127 |
| foregoes | Negative | 0.137 |
| foregone | Negative | 0.109 |

| | | |
|---|---|---|
| forfeit | Negative | −0.158 |
| forfeited | Negative | 0.303 |
| forfeiture | Negative | −0.114 |
| forgery | Negative | 0.058 |
| fraud | Negative | −0.257 |
| fraudulent | Negative | 0.492 |
| fraudulently | Negative | −0.202 |
| frustrated | Negative | −0.490 |
| frustrating | Negative | −0.482 |
| gratuitous | Negative | 0.009 |
| gratuitously | Negative | −0.008 |
| grievances | Negative | 0.278 |
| groundless | Negative | −0.307 |
| guilty | Negative | −0.076 |
| halt | Negative | −0.346 |
| halted | Negative | 0.060 |
| hamper | Negative | −0.062 |
| hampered | Negative | 0.145 |
| hampering | Negative | 0.090 |
| hampers | Negative | −0.094 |
| hardship | Negative | 0.134 |
| harm | Negative | −0.205 |
| harmed | Negative | 0.153 |
| harming | Negative | −0.236 |
| harms | Negative | −0.086 |
| harsh | Negative | −0.290 |
| hazard | Negative | −0.159 |
| hazardous | Negative | 0.020 |
| hazards | Negative | 0.206 |
| hinder | Negative | −0.284 |
| hindered | Negative | 0.184 |
| hindering | Negative | −0.003 |
| hindrance | Negative | 0.042 |
| hostile | Negative | 0.118 |
| hurt | Negative | 0.248 |
| hurting | Negative | −0.229 |
| idle | Negative | −0.393 |
| idled | Negative | 0.187 |
| ignore | Negative | 0.224 |
| ignored | Negative | 0.264 |
| ignores | Negative | −0.084 |
| ignoring | Negative | 0.142 |
| ill | Negative | 0.151 |
| illegal | Negative | 0.054 |
| illiquidity | Negative | −0.480 |
| imbalances | Negative | 0.230 |
| impair | Negative | −0.259 |
| impaired | Negative | 0.074 |
| impairing | Negative | −0.153 |

| | | |
|---|---|---|
| impairment | Negative | −0.088 |
| impairments | Negative | 0.088 |
| impairs | Negative | −0.130 |
| impede | Negative | −0.384 |
| impeded | Negative | 0.195 |
| impeding | Negative | 0.128 |
| impending | Negative | −0.152 |
| imperative | Negative | −0.216 |
| implicated | Negative | −0.177 |
| impossible | Negative | −0.313 |
| imprisonment | Negative | 0.035 |
| improper | Negative | −0.414 |
| improperly | Negative | 0.109 |
| imprudent | Negative | 0.058 |
| inaccuracies | Negative | 0.220 |
| inaccurate | Negative | 0.301 |
| inactivity | Negative | 0.117 |
| inadequacy | Negative | 0.074 |
| inadequate | Negative | 0.072 |
| inappropriate | Negative | 0.100 |
| inappropriately | Negative | 0.047 |
| incapacitated | Negative | −0.061 |
| incidence | Negative | −0.364 |
| incident | Negative | −0.224 |
| incidents | Negative | 0.112 |
| incompatibilities | Negative | 0.036 |
| incompatibility | Negative | −0.015 |
| incomplete | Negative | 0.013 |
| incompletely | Negative | −0.084 |
| inconclusive | Negative | −0.138 |
| inconsistencies | Negative | 0.169 |
| inconsistent | Negative | −0.020 |
| inconsistently | Negative | −0.095 |
| inconvenience | Negative | −0.364 |
| incorrect | Negative | 0.220 |
| incorrectly | Negative | −0.207 |
| indicted | Negative | −0.044 |
| indictment | Negative | 0.110 |
| indictments | Negative | 0.227 |
| inefficiencies | Negative | −0.029 |
| inefficiency | Negative | −0.006 |
| inefficient | Negative | 0.122 |
| inefficiently | Negative | −0.532 |
| ineligible | Negative | −0.036 |
| inevitable | Negative | 0.136 |
| inferior | Negative | −0.069 |
| infringe | Negative | 0.032 |
| infringed | Negative | 0.304 |
| infringement | Negative | 0.398 |

| | | |
|---|---|---|
| infringements | Negative | 0.014 |
| infringes | Negative | −0.236 |
| infringing | Negative | −0.178 |
| injunction | Negative | −0.396 |
| injured | Negative | −0.166 |
| injuries | Negative | 0.202 |
| injury | Negative | 0.067 |
| inquiry | Negative | −0.079 |
| insecure | Negative | 0.356 |
| insolvencies | Negative | 0.022 |
| insolvency | Negative | 0.156 |
| insolvent | Negative | 0.175 |
| instability | Negative | 0.063 |
| insufficient | Negative | 0.067 |
| interference | Negative | 0.257 |
| interfering | Negative | 0.100 |
| intermittent | Negative | 0.055 |
| interrupt | Negative | 0.092 |
| interrupted | Negative | 0.043 |
| interrupting | Negative | −0.102 |
| interruption | Negative | −0.149 |
| interruptions | Negative | 0.212 |
| invalid | Negative | 0.260 |
| invalidate | Negative | 0.141 |
| invalidity | Negative | 0.016 |
| investigate | Negative | 0.272 |
| investigated | Negative | −0.078 |
| investigates | Negative | −0.063 |
| investigating | Negative | −0.238 |
| investigation | Negative | 0.157 |
| investigations | Negative | 0.170 |
| irrecoverable | Negative | 0.088 |
| irregular | Negative | −0.070 |
| irregularities | Negative | −0.187 |
| irreversible | Negative | −0.150 |
| jeopardize | Negative | 0.204 |
| justifiable | Negative | −0.036 |
| knowingly | Negative | −0.045 |
| lack | Negative | 0.316 |
| lacked | Negative | 0.073 |
| lacking | Negative | 0.397 |
| lacks | Negative | 0.688 |
| lag | Negative | 0.438 |
| lagged | Negative | 0.363 |
| lagging | Negative | −0.060 |
| lags | Negative | −0.094 |
| lapse | Negative | 0.245 |
| lapsed | Negative | 0.411 |
| lapses | Negative | 0.278 |

| | | |
|---|---|---|
| lapsing | Negative | 0.099 |
| late | Negative | 0.198 |
| layoff | Negative | −0.141 |
| layoffs | Negative | 0.293 |
| lie | Negative | 0.108 |
| limitation | Negative | −0.024 |
| limitations | Negative | −0.456 |
| lingering | Negative | 0.058 |
| liquidate | Negative | 0.160 |
| liquidated | Negative | 0.136 |
| liquidates | Negative | 0.179 |
| liquidation | Negative | 0.174 |
| liquidations | Negative | 0.134 |
| liquidator | Negative | 0.064 |
| litigation | Negative | −0.063 |
| litigations | Negative | −0.005 |
| lose | Negative | 0.110 |
| loses | Negative | 0.044 |
| losing | Negative | 0.124 |
| loss | Negative | 0.295 |
| losses | Negative | 0.208 |
| lost | Negative | 0.106 |
| malicious | Negative | −0.176 |
| manipulate | Negative | 0.214 |
| manipulated | Negative | −0.262 |
| manipulation | Negative | 0.153 |
| markdown | Negative | 0.293 |
| markdowns | Negative | 0.174 |
| misconduct | Negative | 0.081 |
| misdemeanor | Negative | −0.465 |
| misleading | Negative | 0.243 |
| mismatch | Negative | 0.127 |
| misrepresented | Negative | −0.006 |
| miss | Negative | −0.045 |
| missed | Negative | 0.120 |
| mistake | Negative | 0.335 |
| mistaken | Negative | −0.106 |
| mistakes | Negative | −0.025 |
| misuse | Negative | 0.187 |
| monopoly | Negative | 0.201 |
| moratorium | Negative | −0.070 |
| mothballing | Negative | −0.009 |
| negative | Negative | 0.170 |
| negatively | Negative | 0.092 |
| neglected | Negative | 0.098 |
| negligent | Negative | −0.366 |
| nullification | Negative | −0.071 |
| nullified | Negative | 0.196 |
| nullifies | Negative | −0.156 |

| | | |
|---|---|---|
| objected | Negative | −0.023 |
| objection | Negative | 0.036 |
| objections | Negative | −0.061 |
| obsolete | Negative | −0.117 |
| obstacle | Negative | 0.282 |
| obstacles | Negative | −0.122 |
| obstructing | Negative | 0.166 |
| offence | Negative | 0.094 |
| omission | Negative | −0.009 |
| omits | Negative | 0.108 |
| omitted | Negative | −0.440 |
| onerous | Negative | −0.026 |
| opportunistic | Negative | 0.138 |
| oppose | Negative | −0.045 |
| opposed | Negative | −0.137 |
| opposes | Negative | 0.190 |
| opposing | Negative | 0.067 |
| opposition | Negative | 0.065 |
| outage | Negative | 0.122 |
| outdated | Negative | 0.329 |
| overages | Negative | 0.119 |
| overcapacities | Negative | 0.109 |
| overcapacity | Negative | 0.051 |
| overcharged | Negative | 0.319 |
| overcome | Negative | 0.123 |
| overcoming | Negative | −0.044 |
| overload | Negative | −0.053 |
| overlooked | Negative | 0.069 |
| overruns | Negative | −0.050 |
| overshadowed | Negative | 0.831 |
| overshadowing | Negative | 0.133 |
| overstated | Negative | −0.099 |
| oversupplied | Negative | −0.147 |
| oversupply | Negative | −0.368 |
| overturned | Negative | −0.075 |
| overvalued | Negative | −0.057 |
| penalties | Negative | 0.135 |
| penalty | Negative | −0.153 |
| perpetrated | Negative | 0.654 |
| persist | Negative | −0.003 |
| persisted | Negative | 0.042 |
| persistence | Negative | 0.378 |
| persistent | Negative | −0.128 |
| persistently | Negative | 0.099 |
| persisting | Negative | −0.036 |
| persists | Negative | −0.003 |
| pervasive | Negative | 0.022 |
| plaintiff | Negative | −0.197 |
| plaintiffs | Negative | 0.217 |

| | | |
|---|---|---|
| plea | Negative | 0.027 |
| plead | Negative | 0.235 |
| pleading | Negative | 0.203 |
| pleas | Negative | 0.133 |
| pled | Negative | 0.697 |
| poor | Negative | 0.087 |
| poorly | Negative | −0.318 |
| posing | Negative | 0.024 |
| postpone | Negative | 0.217 |
| postponed | Negative | 0.161 |
| postponement | Negative | −0.115 |
| postponements | Negative | −0.334 |
| postpones | Negative | 0.057 |
| postponing | Negative | 0.370 |
| precipitated | Negative | −0.038 |
| precipitously | Negative | 0.340 |
| preclude | Negative | −0.040 |
| precluded | Negative | 0.305 |
| precludes | Negative | 0.051 |
| precluding | Negative | −0.004 |
| predatory | Negative | 0.021 |
| prejudice | Negative | 0.219 |
| premature | Negative | 0.130 |
| prematurely | Negative | −0.101 |
| pressing | Negative | 0.719 |
| preventing | Negative | 0.051 |
| prevention | Negative | −0.112 |
| prevents | Negative | 0.111 |
| problem | Negative | 0.000 |
| problematic | Negative | −0.080 |
| problems | Negative | 0.093 |
| prolong | Negative | 0.124 |
| prolongation | Negative | 0.015 |
| prolonged | Negative | −0.041 |
| prolonging | Negative | −0.059 |
| prolongs | Negative | 0.293 |
| prosecute | Negative | 0.116 |
| prosecuting | Negative | 0.004 |
| prosecution | Negative | 0.060 |
| prosecutions | Negative | −0.014 |
| protest | Negative | 0.114 |
| protracted | Negative | 0.160 |
| provoke | Negative | 0.008 |
| punished | Negative | 0.250 |
| punitive | Negative | −0.119 |
| purported | Negative | −0.043 |
| purports | Negative | 0.017 |
| question | Negative | 0.737 |
| questionable | Negative | −0.126 |

| | | |
|---|---|---|
| questioned | Negative | 0.040 |
| questioning | Negative | 0.445 |
| questions | Negative | 0.124 |
| rationalization | Negative | 0.246 |
| rationalize | Negative | −0.123 |
| rationalized | Negative | 0.122 |
| rationalizes | Negative | 0.148 |
| rationalizing | Negative | 0.144 |
| reassessment | Negative | 0.243 |
| reassign | Negative | 0.050 |
| reassigning | Negative | 0.142 |
| reassignment | Negative | 0.162 |
| reassigns | Negative | 0.002 |
| recall | Negative | −0.023 |
| recalled | Negative | −0.179 |
| recalling | Negative | 0.058 |
| recession | Negative | 0.743 |
| recessionary | Negative | −0.388 |
| recessions | Negative | −0.060 |
| redacted | Negative | 0.171 |
| refusal | Negative | 0.204 |
| refuse | Negative | 0.077 |
| refused | Negative | −0.267 |
| refuses | Negative | −0.291 |
| refusing | Negative | −0.014 |
| reject | Negative | −0.046 |
| rejected | Negative | 0.181 |
| rejection | Negative | 0.021 |
| rejections | Negative | 0.028 |
| rejects | Negative | −0.114 |
| relinquish | Negative | 0.015 |
| relinquished | Negative | 0.047 |
| relinquishes | Negative | −0.074 |
| relinquishing | Negative | −0.318 |
| relinquishment | Negative | 0.149 |
| reluctance | Negative | 0.246 |
| reluctant | Negative | 0.123 |
| renegotiated | Negative | −0.144 |
| renegotiating | Negative | 0.111 |
| renegotiation | Negative | −0.005 |
| renounce | Negative | −0.157 |
| renounced | Negative | 0.073 |
| resign | Negative | 0.006 |
| resignation | Negative | 0.093 |
| resignations | Negative | 0.689 |
| resigned | Negative | −0.049 |
| resigning | Negative | −0.013 |
| resigns | Negative | −0.029 |
| restate | Negative | 0.166 |

| | | |
|---|---|---|
| restated | Negative | −0.014 |
| restatement | Negative | −0.065 |
| restatements | Negative | −0.077 |
| restates | Negative | 0.036 |
| restructure | Negative | −0.068 |
| restructured | Negative | 0.164 |
| restructures | Negative | 0.118 |
| restructuring | Negative | −0.494 |
| restructurings | Negative | −0.250 |
| revocation | Negative | −0.012 |
| revoke | Negative | −0.109 |
| revoked | Negative | 0.029 |
| revokes | Negative | −0.094 |
| revoking | Negative | 0.684 |
| risky | Negative | 0.174 |
| sabotage | Negative | 0.028 |
| sacrificed | Negative | −0.184 |
| scrutinizing | Negative | −0.368 |
| scrutiny | Negative | 0.222 |
| secrecy | Negative | 0.055 |
| seize | Negative | 0.110 |
| seized | Negative | 0.020 |
| seizing | Negative | 0.174 |
| sentenced | Negative | −0.063 |
| serious | Negative | 0.126 |
| seriously | Negative | −0.160 |
| setback | Negative | −0.292 |
| setbacks | Negative | 0.129 |
| severe | Negative | 0.131 |
| severed | Negative | 0.039 |
| severely | Negative | −0.001 |
| severity | Negative | −0.014 |
| sharply | Negative | −0.167 |
| shocked | Negative | 0.079 |
| shortage | Negative | 0.338 |
| shortages | Negative | 0.082 |
| shortfall | Negative | 0.048 |
| shortfalls | Negative | 0.036 |
| shrinkage | Negative | 0.355 |
| shut | Negative | 0.007 |
| shutdown | Negative | 0.144 |
| shutdowns | Negative | 0.161 |
| shuts | Negative | 0.265 |
| shutting | Negative | 0.186 |
| slippage | Negative | 0.190 |
| slow | Negative | 0.075 |
| slowdown | Negative | 0.178 |
| slowdowns | Negative | 0.044 |
| slowed | Negative | −0.131 |

| | | |
|---|---|---|
| slower | Negative | 0.054 |
| slowing | Negative | −0.084 |
| slowly | Negative | −0.129 |
| slowness | Negative | 0.182 |
| sluggish | Negative | 0.246 |
| sluggishly | Negative | 0.177 |
| sluggishness | Negative | 0.165 |
| solvency | Negative | 0.108 |
| staggering | Negative | −0.063 |
| stagnant | Negative | −0.220 |
| stagnate | Negative | 0.037 |
| stagnated | Negative | 0.401 |
| stagnating | Negative | 0.044 |
| stagnation | Negative | −0.079 |
| standstill | Negative | 0.050 |
| stoppage | Negative | −0.087 |
| stoppages | Negative | 0.163 |
| stopped | Negative | 0.241 |
| stopping | Negative | 0.083 |
| stops | Negative | 0.152 |
| strain | Negative | 0.047 |
| strained | Negative | −0.159 |
| strains | Negative | −0.244 |
| stress | Negative | 0.110 |
| stressed | Negative | 0.045 |
| stresses | Negative | −0.212 |
| stringent | Negative | −0.192 |
| subjected | Negative | −0.331 |
| subjecting | Negative | 0.039 |
| subpoena | Negative | 0.052 |
| subpoenas | Negative | 0.077 |
| sue | Negative | 0.184 |
| sued | Negative | 0.041 |
| sues | Negative | 0.216 |
| suffer | Negative | −0.335 |
| suffered | Negative | −0.044 |
| suffering | Negative | 0.580 |
| suffers | Negative | 0.250 |
| suing | Negative | 0.212 |
| summoned | Negative | −0.340 |
| summons | Negative | −0.039 |
| susceptibility | Negative | −0.022 |
| susceptible | Negative | 0.019 |
| suspect | Negative | 0.041 |
| suspected | Negative | 0.170 |
| suspects | Negative | 0.061 |
| suspend | Negative | 0.011 |
| suspended | Negative | −0.443 |
| suspending | Negative | 0.128 |

| | | |
|---|---|---|
| suspends | Negative | 0.043 |
| suspension | Negative | 0.044 |
| suspensions | Negative | −0.015 |
| suspicion | Negative | −0.235 |
| suspicions | Negative | 0.070 |
| tense | Negative | −0.128 |
| terminate | Negative | −0.432 |
| terminated | Negative | 0.359 |
| terminates | Negative | −0.086 |
| terminating | Negative | 0.032 |
| termination | Negative | 0.185 |
| terminations | Negative | 0.149 |
| testify | Negative | 0.126 |
| threat | Negative | −0.210 |
| threaten | Negative | −0.292 |
| threatened | Negative | 0.035 |
| threatening | Negative | 0.186 |
| threatens | Negative | 0.173 |
| threats | Negative | 0.285 |
| tightening | Negative | 0.106 |
| tolerate | Negative | 0.231 |
| tolerated | Negative | 0.056 |
| tolerates | Negative | −0.167 |
| tortuous | Negative | −0.055 |
| tragedy | Negative | −0.355 |
| tragic | Negative | −0.143 |
| trouble | Negative | 0.147 |
| troubled | Negative | 0.032 |
| turbulence | Negative | −0.186 |
| turmoil | Negative | 0.022 |
| unable | Negative | 0.071 |
| unacceptably | Negative | 0.088 |
| unaccounted | Negative | 0.030 |
| unanticipated | Negative | 0.062 |
| unattractive | Negative | −0.080 |
| unauthorized | Negative | 0.025 |
| unavailability | Negative | −0.030 |
| unavoidable | Negative | −0.151 |
| unaware | Negative | −0.079 |
| uncollectable | Negative | −0.062 |
| uncollectible | Negative | −0.148 |
| uncompetitive | Negative | −0.465 |
| uncontrollable | Negative | 0.349 |
| uncovered | Negative | 0.030 |
| undeliverable | Negative | 0.048 |
| undercut | Negative | 0.036 |
| undercutting | Negative | −0.138 |
| underestimated | Negative | −0.093 |
| underestimation | Negative | −0.465 |

| | | |
|---|---|---|
| undermined | Negative | −0.059 |
| underperformance | Negative | −0.038 |
| underperforming | Negative | 0.463 |
| underutilization | Negative | 0.270 |
| undesirable | Negative | 0.098 |
| undetected | Negative | 0.049 |
| undetermined | Negative | 0.271 |
| undisclosed | Negative | 0.022 |
| undue | Negative | −0.133 |
| unexpected | Negative | −0.094 |
| unexpectedly | Negative | 0.166 |
| unfavorable | Negative | −0.096 |
| unfavourable | Negative | −0.127 |
| unfeasible | Negative | −0.091 |
| unforeseeable | Negative | −0.232 |
| unforeseen | Negative | 0.446 |
| unfortunate | Negative | 0.068 |
| unfortunately | Negative | −0.075 |
| unfounded | Negative | 0.181 |
| unfriendly | Negative | −0.185 |
| unfulfilled | Negative | −0.173 |
| unjust | Negative | 0.094 |
| unjustified | Negative | −0.052 |
| unlawful | Negative | −0.235 |
| unnecessary | Negative | 0.053 |
| unoccupied | Negative | 0.080 |
| unpaid | Negative | −0.046 |
| unplanned | Negative | 0.275 |
| unpredictability | Negative | 0.435 |
| unpredictable | Negative | −0.004 |
| unprofitable | Negative | 0.145 |
| unqualified | Negative | −0.197 |
| unrealistic | Negative | −0.613 |
| unreasonable | Negative | 0.109 |
| unresolved | Negative | −0.354 |
| unrest | Negative | 0.090 |
| unsafe | Negative | −0.542 |
| unsatisfactory | Negative | 0.024 |
| unscheduled | Negative | −0.320 |
| unsold | Negative | −0.026 |
| unstable | Negative | −0.447 |
| unsubstantiated | Negative | −0.097 |
| unsuccessful | Negative | −0.017 |
| unsuitable | Negative | 0.012 |
| unsure | Negative | 0.057 |
| unsustainable | Negative | 0.011 |
| untruthful | Negative | −0.115 |
| unwilling | Negative | 0.110 |
| upset | Negative | 0.162 |

| | | |
|---|---|---|
| urgency | Negative | 0.334 |
| urgent | Negative | −0.175 |
| verdict | Negative | 0.147 |
| victims | Negative | 0.012 |
| violate | Negative | 0.234 |
| violated | Negative | 0.124 |
| violates | Negative | −0.016 |
| violating | Negative | −0.510 |
| violation | Negative | 0.337 |
| violations | Negative | −0.097 |
| violent | Negative | −0.232 |
| voided | Negative | 0.055 |
| volatile | Negative | 0.066 |
| volatility | Negative | 0.049 |
| vulnerability | Negative | 0.189 |
| vulnerable | Negative | 0.003 |
| warning | Negative | −0.204 |
| warnings | Negative | −0.137 |
| weak | Negative | −0.191 |
| weaken | Negative | 0.144 |
| weakened | Negative | 0.148 |
| weakening | Negative | −0.189 |
| weakens | Negative | 0.182 |
| weaker | Negative | 0.059 |
| weakest | Negative | 0.243 |
| weakly | Negative | 0.188 |
| weakness | Negative | −0.013 |
| weaknesses | Negative | −0.193 |
| worse | Negative | −0.052 |
| worsen | Negative | −0.125 |
| worsened | Negative | −0.296 |
| worsening | Negative | 0.034 |
| worst | Negative | 0.172 |
| worthless | Negative | 0.056 |
| writedown | Negative | 0.125 |
| writedowns | Negative | 0.002 |
| writeoff | Negative | 0.106 |
| wrong | Negative | −0.036 |
| wrongdoing | Negative | 0.131 |
| wrongful | Negative | 0.206 |
| wrongly | Negative | −0.187 |

Table C.5: Standardized predictions for all negative terms from the Loughran-McDonald finance-specific word list. The results stem from an LSTM with word embeddings for the regression task with abnormal returns.

*Appendix C.2. Word stems*

| Stem | Label | Predicted score |
|---|---|---|
| achiev | Positive | 0.185 |
| adequ | Positive | 0.287 |
| advanc | Positive | 0.055 |
| advantag | Positive | 0.055 |
| allianc | Positive | 0.173 |
| assur | Positive | −0.069 |
| attain | Positive | 0.164 |
| attract | Positive | 0.494 |
| benefici | Positive | 0.383 |
| benefit | Positive | −0.029 |
| best | Positive | 0.299 |
| better | Positive | 0.046 |
| boom | Positive | 0.035 |
| boost | Positive | 0.134 |
| breakthrough | Positive | 0.104 |
| collabor | Positive | −0.123 |
| confid | Positive | 0.062 |
| construct | Positive | 0.548 |
| creativ | Positive | 0.355 |
| delight | Positive | 0.143 |
| desir | Positive | −0.010 |
| despit | Positive | 0.174 |
| easier | Positive | 0.241 |
| easili | Positive | −0.226 |
| easi | Positive | −0.189 |
| effect | Positive | 0.482 |
| effici | Positive | 0.204 |
| enabl | Positive | 0.045 |
| encourag | Positive | 0.020 |
| enhanc | Positive | 0.102 |
| enjoy | Positive | −0.010 |
| enthusiasm | Positive | −0.090 |
| enthusiast | Positive | 0.141 |
| excel | Positive | 0.009 |
| except | Positive | 0.064 |
| excit | Positive | 0.199 |
| exclus | Positive | 0.234 |
| exemplari | Positive | 0.339 |
| fantast | Positive | 0.243 |
| favor | Positive | 0.162 |
| favorit | Positive | 0.067 |
| friendli | Positive | −0.096 |
| gain | Positive | 0.066 |
| good | Positive | −0.111 |
| great | Positive | 0.338 |

| | | |
|---|---|---|
| greater | Positive | −0.026 |
| greatest | Positive | −0.057 |
| greatli | Positive | −0.373 |
| happili | Positive | 0.124 |
| happi | Positive | 0.242 |
| highest | Positive | 0.498 |
| honor | Positive | −0.025 |
| ideal | Positive | 0.314 |
| impress | Positive | −0.112 |
| improv | Positive | −0.118 |
| incred | Positive | −0.056 |
| inform | Positive | −0.304 |
| innov | Positive | 0.042 |
| insight | Positive | −0.352 |
| integr | Positive | −0.022 |
| invent | Positive | −0.001 |
| inventor | Positive | 0.272 |
| leadership | Positive | 0.414 |
| lead | Positive | −0.146 |
| loyal | Positive | −0.107 |
| lucr | Positive | 0.139 |
| opportun | Positive | 0.256 |
| optimist | Positive | 0.126 |
| outperform | Positive | 0.128 |
| perfect | Positive | 0.331 |
| perfectli | Positive | −0.023 |
| pleasant | Positive | 0.269 |
| pleasantli | Positive | 0.214 |
| pleas | Positive | 0.363 |
| pleasur | Positive | 0.111 |
| popular | Positive | −0.027 |
| posit | Positive | −0.101 |
| premier | Positive | 0.106 |
| prestig | Positive | 0.251 |
| prestigi | Positive | −0.090 |
| proactiv | Positive | 0.119 |
| profit | Positive | −0.029 |
| progress | Positive | 0.167 |
| prosper | Positive | 0.040 |
| rebound | Positive | 0.135 |
| regain | Positive | −0.022 |
| resolv | Positive | 0.404 |
| revolution | Positive | 0.170 |
| reward | Positive | 0.133 |
| satisfact | Positive | −0.106 |
| satisfactorili | Positive | 0.119 |
| satisfactori | Positive | 0.180 |
| satisfi | Positive | 0.213 |
| smooth | Positive | 0.143 |

| | | |
|---|---|---|
| smoothli | Positive | 0.079 |
| solv | Positive | 0.029 |
| spectacular | Positive | 0.267 |
| stabil | Positive | 0.157 |
| stabl | Positive | 0.042 |
| strength | Positive | 0.274 |
| strengthen | Positive | 0.103 |
| strong | Positive | 0.225 |
| stronger | Positive | 0.421 |
| strongest | Positive | −0.387 |
| succeed | Positive | 0.052 |
| succe | Positive | 0.387 |
| success | Positive | −0.008 |
| superior | Positive | 0.416 |
| surpass | Positive | 0.009 |
| transpar | Positive | 0.071 |
| tremend | Positive | −0.120 |
| unparallel | Positive | −0.269 |
| upturn | Positive | 0.186 |
| valuabl | Positive | 0.042 |
| versatil | Positive | −0.054 |
| vibrant | Positive | −0.193 |
| win | Positive | 0.035 |
| winner | Positive | 0.356 |
| worthi | Positive | 0.238 |

Table C.6: Standardized predictions for all positive terms from the Loughran-McDonald finance-specific word list. The results stem from an LSTM with word embeddings for the regression task with abnormal returns. He we specifically perform stemming.

| **Stem** | **Label** | **Predicted score** |
|---|---|---|
| absenc | Negative | −0.137 |
| abus | Negative | 0.022 |
| advers | Negative | 0.032 |
| against | Negative | −0.090 |
| alleg | Negative | −0.322 |
| antitrust | Negative | 0.627 |
| bad | Negative | 0.007 |
| bankruptci | Negative | −0.148 |
| bottleneck | Negative | −0.083 |
| breach | Negative | −0.101 |
| break | Negative | −0.367 |
| breakdown | Negative | −0.054 |
| bridg | Negative | 0.013 |

| | | |
|---|---|---|
| burden | Negative | −0.175 |
| cancel | Negative | 0.067 |
| caution | Negative | −0.007 |
| cautionari | Negative | −0.319 |
| ceas | Negative | −0.138 |
| challeng | Negative | −0.156 |
| claim | Negative | −0.361 |
| close | Negative | −0.255 |
| closur | Negative | −0.008 |
| collaps | Negative | 0.110 |
| complaint | Negative | 0.024 |
| concern | Negative | 0.004 |
| conflict | Negative | −0.158 |
| contract | Negative | 0.111 |
| contrari | Negative | −0.025 |
| correct | Negative | 0.007 |
| crimin | Negative | −0.110 |
| crise | Negative | −0.234 |
| crisi | Negative | −0.174 |
| critic | Negative | −0.024 |
| crucial | Negative | −0.006 |
| culpabl | Negative | −0.012 |
| curtail | Negative | 0.030 |
| cut | Negative | 0.053 |
| cutback | Negative | 0.261 |
| damag | Negative | −0.154 |
| dampen | Negative | 0.190 |
| danger | Negative | 0.035 |
| deadlock | Negative | −0.105 |
| deceit | Negative | 0.156 |
| decept | Negative | −0.023 |
| declin | Negative | −0.071 |
| defamatori | Negative | 0.109 |
| default | Negative | −0.179 |
| defeat | Negative | −0.002 |
| defect | Negative | 0.038 |
| defend | Negative | −0.220 |
| defer | Negative | 0.323 |
| defici | Negative | 0.006 |
| deficit | Negative | 0.104 |
| defraud | Negative | 0.141 |
| defunct | Negative | −0.321 |
| degrad | Negative | −0.366 |
| delay | Negative | 0.246 |
| deliber | Negative | −0.154 |
| delist | Negative | 0.148 |
| demolish | Negative | −0.086 |
| demolit | Negative | −0.031 |
| deni | Negative | 0.158 |

| | | |
|---|---|---|
| deplet | Negative | 0.170 |
| deprec | Negative | 0.008 |
| depress | Negative | −0.010 |
| depriv | Negative | −0.047 |
| destabil | Negative | −0.200 |
| destroy | Negative | 0.204 |
| destruct | Negative | 0.255 |
| detain | Negative | 0.339 |
| detent | Negative | −0.062 |
| deter | Negative | 0.234 |
| deterior | Negative | −0.068 |
| deterr | Negative | 0.259 |
| detract | Negative | 0.210 |
| detriment | Negative | 0.226 |
| devast | Negative | 0.073 |
| deviat | Negative | 0.032 |
| difficult | Negative | −0.002 |
| difficulti | Negative | 0.071 |
| diminish | Negative | 0.060 |
| diminut | Negative | −0.135 |
| disadvantag | Negative | 0.020 |
| disagr | Negative | 0.069 |
| disagre | Negative | 0.113 |
| disappear | Negative | −0.343 |
| disappoint | Negative | −0.173 |
| disapprov | Negative | −0.064 |
| disast | Negative | −0.127 |
| disastr | Negative | 0.039 |
| disciplinari | Negative | 0.150 |
| disclaim | Negative | −0.068 |
| disclos | Negative | 0.033 |
| discontinu | Negative | 0.042 |
| discrep | Negative | −0.450 |
| disgorg | Negative | −0.256 |
| dismiss | Negative | −0.082 |
| displac | Negative | −0.101 |
| dispos | Negative | −0.079 |
| disproport | Negative | −0.020 |
| disproportion | Negative | −0.132 |
| disput | Negative | 0.131 |
| disqualif | Negative | −0.059 |
| disqualifi | Negative | 0.067 |
| disregard | Negative | −0.004 |
| disrupt | Negative | −0.137 |
| dissatisfact | Negative | 0.723 |
| dissent | Negative | 0.008 |
| dissolut | Negative | 0.113 |
| distort | Negative | −0.034 |
| distract | Negative | 0.158 |

| | | |
|---|---|---|
| distress | Negative | 0.009 |
| disturb | Negative | 0.098 |
| divest | Negative | 0.045 |
| divestitur | Negative | 0.178 |
| divulg | Negative | 0.293 |
| doubt | Negative | 0.084 |
| downgrad | Negative | 0.198 |
| downsiz | Negative | 0.058 |
| downtim | Negative | 0.171 |
| downturn | Negative | 0.106 |
| downward | Negative | −0.106 |
| drag | Negative | 0.006 |
| drastic | Negative | −0.304 |
| drawback | Negative | 0.164 |
| drop | Negative | −0.042 |
| drought | Negative | 0.253 |
| dysfunct | Negative | −0.019 |
| eas | Negative | −0.056 |
| embarrass | Negative | 0.038 |
| encumb | Negative | −0.085 |
| encumbr | Negative | −0.040 |
| endang | Negative | 0.110 |
| enjoin | Negative | 0.063 |
| erod | Negative | −0.174 |
| eros | Negative | −0.101 |
| erron | Negative | 0.262 |
| error | Negative | −0.203 |
| escal | Negative | −0.036 |
| exacerb | Negative | 0.124 |
| exagger | Negative | 0.300 |
| excess | Negative | −0.018 |
| exoner | Negative | 0.218 |
| exploit | Negative | 0.047 |
| expos | Negative | 0.025 |
| expuls | Negative | 0.188 |
| fail | Negative | −0.025 |
| failur | Negative | −0.172 |
| 0 | Negative | 0.000 |
| fault | Negative | 0.027 |
| faulti | Negative | −0.121 |
| fear | Negative | 0.137 |
| feloni | Negative | −0.287 |
| fictiti | Negative | −0.418 |
| fine | Negative | 0.129 |
| fire | Negative | 0.059 |
| flaw | Negative | 0.090 |
| forbid | Negative | −0.223 |
| forbidden | Negative | 0.006 |
| forc | Negative | 0.163 |

| | | |
|---|---|---|
| forego | Negative | 0.162 |
| foregon | Negative | 0.093 |
| forfeit | Negative | −0.016 |
| forfeitur | Negative | −0.042 |
| forgeri | Negative | 0.059 |
| fraud | Negative | −0.227 |
| fraudul | Negative | 0.220 |
| frustrat | Negative | −0.468 |
| gratuit | Negative | −0.053 |
| grievanc | Negative | 0.325 |
| groundless | Negative | −0.291 |
| guilti | Negative | −0.098 |
| halt | Negative | −0.184 |
| hamper | Negative | 0.016 |
| hardship | Negative | 0.075 |
| harm | Negative | −0.098 |
| harsh | Negative | −0.260 |
| hazard | Negative | 0.101 |
| hinder | Negative | 0.049 |
| hindranc | Negative | 0.013 |
| hostil | Negative | 0.138 |
| hurt | Negative | −0.090 |
| idl | Negative | −0.116 |
| ignor | Negative | 0.119 |
| ill | Negative | 0.125 |
| illeg | Negative | 0.106 |
| illiquid | Negative | −0.451 |
| imbal | Negative | 0.201 |
| impair | Negative | −0.069 |
| imped | Negative | −0.036 |
| impend | Negative | −0.209 |
| imper | Negative | −0.283 |
| implic | Negative | −0.150 |
| imposs | Negative | −0.353 |
| imprison | Negative | 0.011 |
| improp | Negative | −0.392 |
| improperli | Negative | 0.097 |
| imprud | Negative | 0.088 |
| inaccuraci | Negative | 0.261 |
| inaccur | Negative | 0.333 |
| inact | Negative | 0.176 |
| inadequaci | Negative | 0.116 |
| inadequ | Negative | 0.068 |
| inappropri | Negative | 0.108 |
| incapacit | Negative | −0.037 |
| incid | Negative | −0.131 |
| incompat | Negative | 0.078 |
| incomplet | Negative | −0.091 |
| inconclus | Negative | −0.104 |

| | | |
|---|---|---|
| inconsist | Negative | −0.087 |
| inconveni | Negative | −0.423 |
| incorrect | Negative | 0.113 |
| incorrectli | Negative | −0.191 |
| indict | Negative | 0.084 |
| ineffici | Negative | −0.089 |
| inelig | Negative | 0.056 |
| inevit | Negative | 0.171 |
| inferior | Negative | 0.015 |
| infring | Negative | −0.031 |
| injunct | Negative | −0.392 |
| injur | Negative | −0.169 |
| injuri | Negative | 0.118 |
| inquiri | Negative | −0.067 |
| insecur | Negative | 0.387 |
| insolv | Negative | 0.110 |
| instabl | Negative | 0.045 |
| insuffici | Negative | 0.133 |
| interfer | Negative | 0.227 |
| interf | Negative | 0.163 |
| intermitt | Negative | 0.077 |
| interrupt | Negative | 0.011 |
| invalid | Negative | 0.289 |
| investig | Negative | 0.081 |
| irrecover | Negative | 0.035 |
| irregular | Negative | −0.240 |
| irrevers | Negative | −0.229 |
| jeopard | Negative | 0.251 |
| justifi | Negative | −0.079 |
| knowingli | Negative | −0.021 |
| lack | Negative | 0.352 |
| lag | Negative | 0.140 |
| laps | Negative | 0.202 |
| late | Negative | 0.192 |
| layoff | Negative | 0.079 |
| lie | Negative | 0.075 |
| limit | Negative | −0.188 |
| linger | Negative | 0.067 |
| liquid | Negative | 0.140 |
| litig | Negative | 0.058 |
| lose | Negative | 0.284 |
| loss | Negative | 0.339 |
| lost | Negative | 0.155 |
| malici | Negative | −0.136 |
| manipul | Negative | 0.030 |
| markdown | Negative | 0.243 |
| misconduct | Negative | 0.077 |
| misdemeanor | Negative | −0.458 |
| mislead | Negative | 0.230 |

| | | |
|---|---|---|
| mismatch | Negative | 0.183 |
| misrepres | Negative | 0.022 |
| miss | Negative | 0.088 |
| mistak | Negative | 0.154 |
| mistaken | Negative | −0.117 |
| misus | Negative | 0.191 |
| monopoli | Negative | 0.136 |
| moratorium | Negative | −0.088 |
| mothbal | Negative | 0.029 |
| neg | Negative | 0.062 |
| neglect | Negative | 0.193 |
| neglig | Negative | −0.401 |
| nullif | Negative | −0.113 |
| nullifi | Negative | 0.039 |
| object | Negative | −0.070 |
| obsolet | Negative | −0.116 |
| obstacl | Negative | 0.102 |
| obstruct | Negative | 0.183 |
| offenc | Negative | 0.100 |
| omiss | Negative | −0.036 |
| omit | Negative | −0.238 |
| oner | Negative | −0.064 |
| opportunist | Negative | 0.106 |
| oppos | Negative | 0.013 |
| opposit | Negative | 0.014 |
| outag | Negative | 0.125 |
| outdat | Negative | 0.271 |
| overag | Negative | 0.019 |
| overcapac | Negative | 0.116 |
| overcharg | Negative | 0.337 |
| overcom | Negative | 0.078 |
| overload | Negative | −0.118 |
| overlook | Negative | −0.003 |
| overrun | Negative | −0.024 |
| overshadow | Negative | 0.523 |
| overst | Negative | −0.085 |
| oversuppli | Negative | −0.206 |
| overturn | Negative | −0.108 |
| overvalu | Negative | −0.034 |
| penalti | Negative | −0.018 |
| perpetr | Negative | 0.606 |
| persist | Negative | 0.093 |
| pervas | Negative | 0.019 |
| plaintiff | Negative | 0.026 |
| plea | Negative | 0.089 |
| plead | Negative | 0.255 |
| pled | Negative | 0.718 |
| poor | Negative | 0.059 |
| poorli | Negative | −0.208 |

| | | |
|---|---|---|
| pose | Negative | 0.010 |
| postpon | Negative | 0.036 |
| precipit | Negative | 0.222 |
| preclud | Negative | 0.102 |
| predatori | Negative | 0.045 |
| prejudic | Negative | 0.195 |
| prematur | Negative | 0.088 |
| press | Negative | 0.759 |
| prevent | Negative | 0.049 |
| problem | Negative | 0.037 |
| problemat | Negative | −0.228 |
| prolong | Negative | 0.057 |
| prosecut | Negative | 0.126 |
| protest | Negative | 0.109 |
| protract | Negative | 0.122 |
| provok | Negative | 0.079 |
| punish | Negative | 0.182 |
| punit | Negative | −0.043 |
| purport | Negative | 0.012 |
| question | Negative | 0.266 |
| ration | Negative | 0.093 |
| reassess | Negative | 0.345 |
| reassign | Negative | 0.147 |
| recal | Negative | 0.054 |
| recess | Negative | 0.348 |
| recessionari | Negative | −0.367 |
| redact | Negative | 0.185 |
| refus | Negative | −0.139 |
| reject | Negative | 0.018 |
| relinquish | Negative | 0.066 |
| reluct | Negative | 0.207 |
| renegoti | Negative | 0.043 |
| renounc | Negative | 0.036 |
| resign | Negative | 0.131 |
| restat | Negative | 0.019 |
| restructur | Negative | −0.175 |
| revoc | Negative | −0.106 |
| revok | Negative | 0.153 |
| riski | Negative | 0.150 |
| sabotag | Negative | 0.046 |
| sacrif | Negative | −0.194 |
| scrutin | Negative | −0.401 |
| scrutini | Negative | 0.185 |
| secreci | Negative | 0.048 |
| seiz | Negative | 0.091 |
| sentenc | Negative | −0.051 |
| seriou | Negative | 0.061 |
| serious | Negative | −0.233 |
| setback | Negative | 0.053 |

| | | |
|---|---|---|
| sever | Negative | 0.112 |
| sharpli | Negative | −0.147 |
| shock | Negative | 0.044 |
| shortag | Negative | 0.311 |
| shortfal | Negative | −0.029 |
| shrinkag | Negative | 0.423 |
| shut | Negative | 0.146 |
| shutdown | Negative | 0.161 |
| slippag | Negative | 0.163 |
| slow | Negative | 0.053 |
| slowdown | Negative | 0.111 |
| slower | Negative | 0.075 |
| slowli | Negative | −0.137 |
| sluggish | Negative | 0.141 |
| sluggishli | Negative | 0.307 |
| solvenc | Negative | 0.059 |
| stagger | Negative | 0.009 |
| stagnant | Negative | −0.149 |
| stagnat | Negative | 0.064 |
| standstil | Negative | 0.072 |
| stoppag | Negative | −0.025 |
| stop | Negative | 0.181 |
| strain | Negative | −0.061 |
| stress | Negative | 0.042 |
| stringent | Negative | −0.134 |
| subject | Negative | −0.150 |
| subpoena | Negative | 0.154 |
| sue | Negative | 0.180 |
| su | Negative | 0.103 |
| suffer | Negative | 0.128 |
| summon | Negative | −0.288 |
| suscept | Negative | −0.129 |
| suspect | Negative | 0.142 |
| suspend | Negative | −0.083 |
| suspens | Negative | 0.028 |
| suspicion | Negative | −0.046 |
| tens | Negative | −0.141 |
| termin | Negative | 0.050 |
| testifi | Negative | 0.196 |
| threat | Negative | 0.025 |
| threaten | Negative | 0.072 |
| tighten | Negative | 0.094 |
| toler | Negative | 0.031 |
| tortuou | Negative | −0.087 |
| tragedi | Negative | −0.280 |
| tragic | Negative | −0.162 |
| troubl | Negative | −0.010 |
| turbul | Negative | −0.163 |
| turmoil | Negative | −0.087 |

| | | |
|---|---|---|
| unabl | Negative | 0.095 |
| unaccept | Negative | 0.160 |
| unaccount | Negative | 0.152 |
| unanticip | Negative | 0.122 |
| unattract | Negative | −0.183 |
| unauthor | Negative | 0.011 |
| unavail | Negative | −0.022 |
| unavoid | Negative | −0.022 |
| unawar | Negative | −0.020 |
| uncollect | Negative | −0.073 |
| uncompetit | Negative | −0.449 |
| uncontrol | Negative | 0.347 |
| uncov | Negative | 0.024 |
| undeliver | Negative | 0.051 |
| undercut | Negative | −0.095 |
| underestim | Negative | −0.199 |
| undermin | Negative | −0.048 |
| underperform | Negative | 0.185 |
| underutil | Negative | 0.250 |
| undesir | Negative | 0.101 |
| undetect | Negative | −0.012 |
| undetermin | Negative | 0.249 |
| undisclos | Negative | 0.072 |
| undu | Negative | −0.066 |
| unexpect | Negative | −0.093 |
| unexpectedli | Negative | 0.190 |
| unfavor | Negative | −0.070 |
| unfavour | Negative | −0.104 |
| unfeas | Negative | −0.105 |
| unforese | Negative | −0.171 |
| unforeseen | Negative | 0.453 |
| unfortun | Negative | 0.062 |
| unfound | Negative | 0.089 |
| unfriendli | Negative | −0.107 |
| unfulfil | Negative | −0.214 |
| unjust | Negative | 0.102 |
| unjustifi | Negative | −0.059 |
| unlaw | Negative | −0.257 |
| unnecessari | Negative | 0.069 |
| unoccupi | Negative | 0.041 |
| unpaid | Negative | −0.059 |
| unplan | Negative | 0.240 |
| unpredict | Negative | 0.173 |
| unprofit | Negative | 0.114 |
| unqualifi | Negative | −0.192 |
| unrealist | Negative | −0.666 |
| unreason | Negative | 0.133 |
| unresolv | Negative | −0.337 |
| unrest | Negative | 0.070 |

| | | |
|---|---|---|
| unsaf | Negative | −0.570 |
| unsatisfactori | Negative | 0.050 |
| unschedul | Negative | −0.336 |
| unsold | Negative | −0.030 |
| unstabl | Negative | −0.404 |
| unsubstanti | Negative | −0.061 |
| unsuccess | Negative | −0.109 |
| unsuit | Negative | 0.007 |
| unsur | Negative | 0.114 |
| unsustain | Negative | 0.066 |
| untruth | Negative | 0.001 |
| unwil | Negative | 0.042 |
| upset | Negative | 0.113 |
| urgenc | Negative | 0.324 |
| urgent | Negative | −0.116 |
| verdict | Negative | 0.087 |
| victim | Negative | −0.019 |
| violat | Negative | 0.087 |
| violent | Negative | −0.276 |
| void | Negative | 0.046 |
| volatil | Negative | 0.056 |
| vulner | Negative | 0.020 |
| warn | Negative | −0.231 |
| weak | Negative | −0.134 |
| weaken | Negative | 0.128 |
| weaker | Negative | 0.070 |
| weakest | Negative | 0.291 |
| weakli | Negative | 0.131 |
| wors | Negative | −0.080 |
| worsen | Negative | −0.193 |
| worst | Negative | 0.108 |
| worthless | Negative | 0.145 |
| writedown | Negative | 0.064 |
| writeoff | Negative | 0.048 |
| wrong | Negative | 0.063 |
| wrongdo | Negative | 0.113 |
| wrongli | Negative | −0.217 |

Table C.7: Standardized predictions for all negative terms from the Loughran-McDonald finance-specific word list. The results stem from an LSTM with word embeddings for the regression task with abnormal returns. He we specifically perform stemming.

## References

[1] T. I. Loughran, B. McDonald, When is a liability not a liability? textual analysis, dictionaries, and 10-Ks, The Journal of Finance 66 (2011) 35–65.
